# Supplementary material for: Cross Space and Time: A Spatio-Temporal Unitized Model for Traffic Flow Forecasting
Source: arXiv:2411.09251 source file (2024-11-14)
Supplement: Supplementary file 1 [file 06_appendix.tex]

\newpage
\appendix
\begin{table*}[ht]
  \centering
  \caption{For 3, 6, and 12 time steps the performance is recorded in detail.}
    \begin{tabular}{c|c|ccc|ccc|ccc|}
    \multirow{2}[3]{*}{\textbf{Data}} & \multirow{2}[3]{*}{\textbf{Models}} & \multicolumn{3}{c|}{15 min} & \multicolumn{3}{c|}{30min} & \multicolumn{3}{c|}{60min} \\
\cmidrule{3-11}          &       & \textbf{MAE} & \textbf{RMSE} & \textbf{MAPE} & \textbf{MAE} & \textbf{RMSE} & \textbf{MAPE} & \textbf{MAE} & \textbf{RMSE} & \textbf{MAPE} \\
    \midrule
    \multirow{10}[10]{*}{\begin{sideways}METR-LA\end{sideways}} & STGCN & 2.7974 & 5.3959 & 0.0736 & 3.1635 & 6.4307 & 0.0884 & 3.5743 & 7.4630 & 0.1049 \\
          & STGCN-A & \textbf{2.7800} & \textbf{5.3759} & \textbf{0.0733} & \textbf{3.1389} & \textbf{6.4054} & \textbf{0.0877} & \textbf{3.5418} & \textbf{7.4321} & \textbf{0.1040} \\
\cmidrule{2-11}          & GWNET & 2.7638 & 5.2634 & 0.0721 & 3.1571 & 6.2805 & 0.0876 & 3.6135 & 7.3723 & 0.1057 \\
          & GWNET-A & \textbf{2.7445} & \textbf{5.2534} & \textbf{0.0714} & \textbf{3.1312} & \textbf{6.2632} & \textbf{0.0860} & \textbf{3.5822} & \textbf{7.3494} & \textbf{0.1033} \\
\cmidrule{2-11}          & AGCRN & 2.8359 & 5.4916 & 0.0761 & 3.1908 & 6.4744 & 0.0900 & 3.5391 & 7.3617 & 0.1031 \\
          & AGCRN-A & 2.8362 & 5.5076 & \textbf{0.0755} & \textbf{3.1852} & \textbf{6.4673} & \textbf{0.0896} & \textbf{3.5378} & \textbf{7.3458} & \textbf{0.1031} \\
\cmidrule{2-11}          & LSTM  & 2.9889 & 5.8662 & 0.0799 & 3.5775 & 7.2127 & 0.1027 & 4.4031 & 8.8507 & 0.1362 \\
          & LSTM-A & \textbf{2.9888} & 5.8839 & \textbf{0.0794} & 3.5786 & 7.2304 & \textbf{0.1025} & 4.4056 & 8.8762 & \textbf{0.1362} \\
\cmidrule{2-11}          & D2STGNN & 2.7192 & 5.1986 & 0.0707 & 3.0506 & 6.1443 & 0.0846 & 3.4485 & 7.1852 & 0.1004 \\
          & D2STGNN-A & 2.7202 & \textbf{5.1838} & 0.0708 & 3.0513 & \textbf{6.1335} & \textbf{0.0843} & \textbf{3.4462} & \textbf{7.1685} & \textbf{0.0997} \\
    \midrule
    \midrule
    \multirow{10}[10]{*}{\begin{sideways}PEMSBAY\end{sideways}} & STGCN & 1.4152 & 2.9129 & 0.0305 & 1.7370 & 3.8352 & 0.0397 & 2.0427 & 4.6089 & 0.0481 \\
          & STGCN-A & \textbf{1.3930} & \textbf{2.8830} & \textbf{0.0301} & \textbf{1.7134} & \textbf{3.8219} & \textbf{0.0394} & \textbf{1.9992} & \textbf{4.5491} & \textbf{0.0477} \\
\cmidrule{2-11}          & GWNET & 1.3443 & 2.8179 & 0.0281 & 1.6937 & 3.7616 & 0.0380 & 2.0399 & 4.5826 & 0.0480 \\
          & GWNET-A & \textbf{1.3395} & \textbf{2.8110} & \textbf{0.0280} & \textbf{1.6838} & 3.7620 & \textbf{0.0379} & \textbf{2.0247} & 4.5835 & 0.0481 \\
\cmidrule{2-11}          & AGCRN & 1.3684 & 2.8559 & 0.0293 & 1.7093 & 3.7831 & 0.0392 & 2.0168 & 4.5350 & 0.0482 \\
          & AGCRN-A & 1.3731 & 2.8582 & 0.0295 & 1.7110 & 3.7953 & 0.0393 & \textbf{2.0044} & 4.5174 & \textbf{0.0477} \\
\cmidrule{2-11}          & LSTM  & 1.4135 & 3.0365 & 0.0297 & 1.8622 & 4.2433 & 0.0426 & 2.3802 & 5.4494 & 0.0592 \\
          & LSTM-A & \textbf{1.4082} & \textbf{3.0236} & \textbf{0.0296} & \textbf{1.8535} & \textbf{4.2220} & \textbf{0.0422} & \textbf{2.3752} & \textbf{5.4144} & \textbf{0.0590} \\
\cmidrule{2-11}          & D2STGNN & 1.3655 & 2.8104 & 0.0301 & 1.7162 & 3.7549 & 0.0412 & 2.0162 & 4.4978 & 0.0492 \\
          & D2STGNN-A & \textbf{1.3600} & \textbf{2.7933} & \textbf{0.0295} & 1.7190 & \textbf{3.7315} & \textbf{0.0410} & 2.0204 & \textbf{4.4903} & \textbf{0.0488} \\
    \midrule
    \midrule
    \multirow{10}[10]{*}{\begin{sideways}PEMS03\end{sideways}} & STGCN & 15.9759 & 26.6721 & 0.1744 & 17.0025 & 28.5349 & 0.1795 & 19.2868 & 32.0878 & 0.2012 \\
          & STGCN-A & \textbf{15.6705} & \textbf{26.1664} & \textbf{0.1672} & \textbf{16.7824} & \textbf{28.3081} & \textbf{0.1735} & \textbf{18.8378} & \textbf{31.7414} & \textbf{0.1887} \\
\cmidrule{2-11}          & GWNET & 13.6307 & 22.9990 & 0.1404 & 14.8984 & 25.2513 & 0.1534 & 17.0542 & 28.5455 & 0.1720 \\
          & GWNET-A & 13.7453 & 23.3552 & 0.1463 & 15.0706 & 25.6562 & 0.1625 & 17.2813 & 29.0168 & 0.1757 \\
\cmidrule{2-11}          & AGCRN & 14.4073 & 25.0248 & 0.1519 & 15.6179 & 27.2081 & 0.1582 & 17.3809 & 30.0750 & 0.1789 \\
          & AGCRN-A & \textbf{14.3017} & \textbf{24.6846} & \textbf{0.1461} & \textbf{15.5948} & \textbf{27.0472} & \textbf{0.1575} & \textbf{17.2572} & \textbf{29.7586} & \textbf{0.1724} \\
\cmidrule{2-11}          & LSTM  & 14.6913 & 24.7252 & 0.1414 & 16.5229 & 27.7032 & 0.1559 & 19.9628 & 32.7821 & 0.1903 \\
          & LSTM-A & 14.7535 & 24.8591 & 0.1474 & 16.6379 & 27.9512 & 0.1630 & 20.1120 & 33.1720 & 0.1909 \\
\cmidrule{2-11}          & D2STGNN & 14.2669 & 23.9886 & 0.1385 & 15.6441 & 26.3575 & 0.1483 & 18.1813 & 30.1904 & 0.1691 \\
          & D2STGNN-A & \textbf{14.2145} & \textbf{23.9346} & 0.1487 & \textbf{15.6118} & \textbf{26.3396} & 0.1590 & \textbf{18.0764} & \textbf{29.9842} & 0.1785 \\
    \midrule
    \midrule
    \multirow{10}[10]{*}{\begin{sideways}PEMS04\end{sideways}} & STGCN & 19.6829 & 30.6939 & 0.1427 & 20.6435 & 32.2766 & 0.1484 & 22.3433 & 34.8944 & 0.1587 \\
          & STGCN-A & \textbf{19.5046} & \textbf{30.4004} & \textbf{0.1432} & \textbf{20.3919} & \textbf{31.9313} & \textbf{0.1474} & \textbf{22.0309} & \textbf{34.5022} & \textbf{0.1556} \\
\cmidrule{2-11}          & GWNET & 18.5208 & 29.5408 & 0.1284 & 19.8411 & 31.3823 & 0.1388 & 22.0469 & 34.2759 & 0.1589 \\
          & GWNET-A & \textbf{18.1948} & \textbf{29.1417} & 0.1291 & \textbf{19.3375} & \textbf{30.7651} & \textbf{0.1379} & \textbf{21.2113} & \textbf{33.3251} & \textbf{0.1527} \\
\cmidrule{2-11}          & AGCRN & 18.1535 & 29.3661 & 0.1271 & 18.9619 & 30.8779 & 0.1317 & 20.1546 & 32.7439 & 0.1424 \\
          & AGCRN-A & 18.2142 & \textbf{29.3064} & 0.1284 & \textbf{19.0631} & \textbf{30.7679} & 0.1346 & 20.3331 & \textbf{32.7270} & 0.1428 \\
\cmidrule{2-11}          & LSTM  & 19.7301 & 31.3637 & 0.1338 & 22.0191 & 34.8805 & 0.1503 & 26.5360 & 41.5353 & 0.1829 \\
          & LSTM-A & 19.7760 & 31.3665 & 0.1368 & 22.0613 & 34.8875 & 0.1523 & 26.5962 & 41.5690 & 0.1869 \\
\cmidrule{2-11}          & D2STGNN & 19.0218 & 29.9526 & 0.1463 & 20.3994 & 31.9117 & 0.1556 & 22.8509 & 35.2251 & 0.1733 \\
          & D2STGNN-A & 19.5439 & 30.8305 & \textbf{0.1396} & 21.0731 & 33.0070 & \textbf{0.1499} & 23.9331 & 36.7999 & \textbf{0.1705} \\
    \bottomrule
    \end{tabular}%
  \label{tab:addlabel}%
\end{table*}%
